# Supplementary material for: A Fast Randomized Algorithm for Massive Text Normalization
Source: arXiv:2110.03024 source file (2021-10-06)
Supplement: Supplementary file 1 [file appendix.tex]

\section{Detailed Steps of Locality-Sensitive Hashing for Words}
\label{sec:detailed-lsh-word}
\begin{figure}[!ht]
\centering
\includegraphics[width=1.0\linewidth]{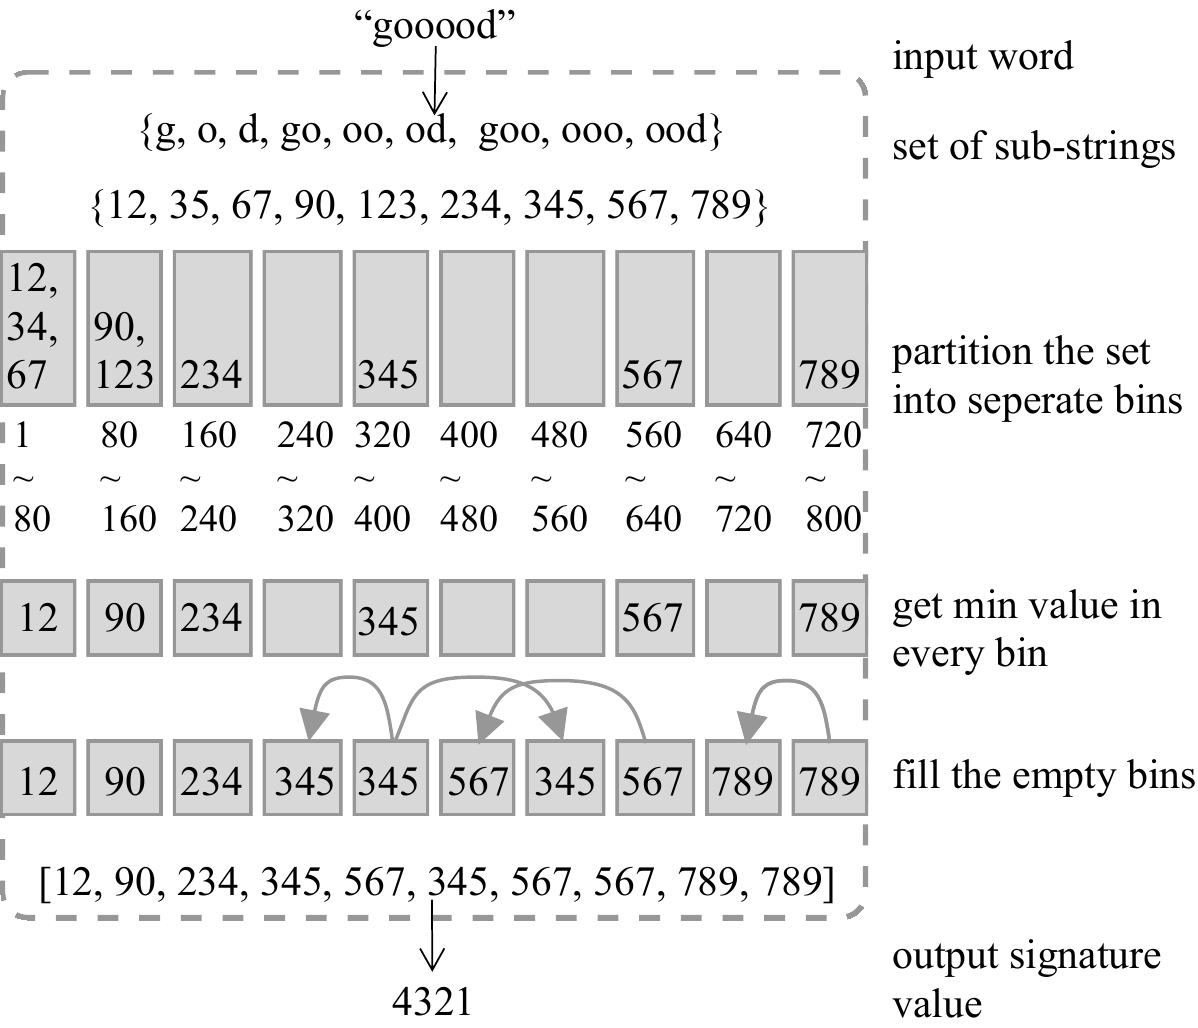}
\caption{An overview of hashing a word into a signature value by LSH. The input word is a sequence of characters and will apply the slicing method with \texttt{CHARLENS} for getting a set of substrings. Then, we use a 2-universal hash function to convert a string into a numerical (integer) value. Finally, we apply the min-wise hashing for the integer values to get a signature value of the input word.}
\label{fig:appendix-lsh}
\end{figure}

The detailed LSH algorithm is composed of several steps as shown in Figure~\ref{fig:appendix-lsh}. First, a word of $n$ characters $w=c_1c_2\cdots c_n$, will be sliced into a set of substrings $\mathcal{S}(w)$: 
\begin{equation*}
\mathcal{S}(w)=\{c_i\}_{i=1}^n\cup\{c_ic_{i+1}\}_{i=1}^{n-1}\cdots\cup\{c_1c_2\cdots c_n\} 
\end{equation*}
Here, $\mathcal{S}(w)$ is the union of character ngram sets. For instance, the substrings set of word ``good'' is: $	\mathcal{S}(\text{good})=\{g,o,d\}\cup\{go,oo,od\}\cup\{goo, ood\}\cup\{good\}$.
In our experiments, we introduce a hyper-parameter $\texttt{CHARLENS}$ to denote which substrings will be included in the set. For example, $\texttt{CHARLENS}=[1,3,5]$ means that the character-level unigram, trigram and 5-gram sets will be included into the overall set $S(w)$. 
Here, for the substring length is longer than the input word length, its N-gram set is defined to be $\emptyset$. Using the above example of $\texttt{CHARLENS}$ setting, for word ``good'', we have: $\mathcal{S}(good)=\{g,o,d\}\cup\{goo, ood\}$.

After obtaining the substring set, we use a hash function $h$ from a 2-universal hash family $\mathcal{H}$ to map every substring into a large universe $U$. The idea is to map every input string uniformly in the large universe $U$ with low collision probability. In our experiments, we use the hash function SHA256.

Next, we use one permutation hashing~\cite{li2012one} to hash the output of above step. We partition the universe $U$ into bins and the set of hashed integers will be correspondingly partitioned. For example, in Figure~\ref{fig:appendix-lsh}, the universe $U=800$ is partitioned into $10$ bins: $[1,80), [80,160), \dots$, $[720,800]$. Those integers $(12, 32, 56, 78)$ inside the first range will be put into the first bin, and the other integers will be partitioned correspondingly. Afterward, for those non-empty bins, we only preserve the minimum value for the bin. For example, for the first bin, we would only preserve the minimum value of $12$. 
 
One existing issue of one permutation hashing is that we cannot have a signature for those empty bins. \citet{DBLP:conf/icml/Shrivastava17} proposes to borrow the signature value in the neighboring bins into the empty bin. In particular, for a given empty bin, we will flip a coin and borrow the first non-empty bin value from either the left or the right. This borrowing process is known as \emph{densification}. After this densification operation, we obtain an array of signature values to represent the input word $w$.

Next, we randomly hash the signature array $[s_1,\cdots,s_m]$ into an integer in another universe $U'$. Here, we need another hash function $h'$ from the 2-universal hash family $\mathcal{H}$ that recursively hashes the array of signature values into one element. Each step takes the sum of the current signature value $s_i$ and the hashed value of the previous step $o_{i-1}$ as input. It will then output the hashed value for the current step: $o_i=h'(s_i+o_{i-1})$, where we use the last element value $o_m$ as the signature value for the input word $w$. We show the detailed process of mapping an input word into a signature in the universe $U'$ in Figure~\ref{fig:appendix-lsh}.

Given two words, $w_i$ and $w_j$, the probability of the words having the same signature value is proportional to the Jaccard similarity of these two words. Hence, we make the assumption that all words grouped together via their signature value are lexically similar (as shown in Figure~\ref{fig:whole}). These grouped words usually are the variant of one canonical representation, which we call the \emph{pivot}. 
In this work, we use this pivot to replace all of the grouped words to normalize the text data.

\section{Error Analysis Proof}
\label{sec:error-proof}
The primary tool for our analysis will be the following Chernoff bounds~\cite{mitzenmacher2017}, which we can apply since the weight of each edge is the sum of independent indicator random variables.
\begin{equation}
\begin{aligned}
Pr[X &\le (1-\delta) T p] \le \exp\left(\frac{-Tp \delta^2}{2}\right), \\
Pr[X &\ge (1+\delta) T p] \le \exp\left(\frac{-Tp\delta^2}{3}\right).
\end{aligned}  
\end{equation}
where $X$ is the weight of a particular edge and $\delta \in (0, 1]$.
\begin{proposition}[False Positive Probability]
Fix a node $w_i$. The probability that FLAN will connect $w_i$ to a node in a cluster $c$ where $c \ne C(w_i)$ is at most $|c|\exp\left(\frac{-T(q-\alpha)^2}{3q}\right)$. $|c|$ is the size of cluster $c$.
\end{proposition}
\begin{proof}
Recall that $e(w_i, w_j)$ denotes the weight assigned to edge $(w_i, w_j)$ by FLAN. Using a Chernoff bound and a union bound, we note that 
\begin{align*}
Pr[\exists w_j \in c&,  (w_i, w_j) \in E] \\
&\le \sum_{j=1}^{|c|} Pr\left[e(w_i, w_j) \ge \alpha T\right] \\
&\le |c|\exp\left(\frac{-T(q-\alpha)^2}{3q}\right)
\end{align*}
where the second inequality follows from setting $\delta = \alpha/q - 1$.
\end{proof}

The above proposition implies that the probability of a false positive event decreases exponentially with more repetitions $T$. As a practical illustration of the power of this bound, if we take $q=0.05, T=10, \alpha=1/2,$ and $|c|=100$, we find that the probability of this bad event is at most $0.000014$.% \cdot 10^{-5}$.
\begin{proposition}[False Negative Probability]
Fix a node $w_i$. The probability that FLAN will not add an edge from $w_i$ to any of the other nodes in $c=C(w_i)$ is at most $\exp\left(\frac{-|c|T (p-\alpha)^2}{2p}\right)$.
\end{proposition}

\begin{proof}
We note that $w_i$ will not share edge with some other word $w_k \in c$ in the FLAN graph if the edge weight is smaller than $\alpha T$ after applying $T$ repetitions. By another Chernoff bound and the fact that the presence of each edge is an independent event, we have that
\begin{align*}
Pr&\left[\forall w_k \in c, (w_i, w_k) \notin E\right] \\
&= \prod_{k=1}^{|c|} Pr[e(w_i, w_k) \le \alpha T] \\
&\le \exp\left(\frac{-|c|T (p-\alpha)^2}{2p}\right)
\end{align*}
where the second inequality follows from setting $\delta = 1 - \alpha/p$.
\end{proof}

\section{Experimental Configurations}
\label{sec:configure}
\subsection{Implementation Details}
For comparison fairness, we use the same procedure of feeding the inputs into and extracting the outputs from the algorithms. In addition, we use parallelism to address computational bottlenecks in the two methods, albeit in different ways. In FLAN, we use every process to run one repetition of the LSH algorithms. In spell-correction, we let every process do spell-correction for a batch of the words. For the \texttt{autocorrect} and Hunspell libraries, they apply one and two steps of operation (i.e., replace, delete, replace and insert) for every input word. For all the word variants in the dictionary, it outputs a word with highest frequency.

Our FLAN algorithm also involve with a a hyper-parameter $\texttt{CHARLENS}$, which is introduced to denote which substrings will be included in the set $\mathcal{S}(w)$. For example, $\texttt{CHARLENS}=[1,3]$ means that the character-level unigram and trigram sets will be included into the overall set $S(w)$. 
Here, for the substring length is longer than the input word length, its N-gram set is defined to be $\emptyset$.

For the hyper-parameters in our experiments, we set \texttt{CHARLEN} to be $[1,2,3,4,5,6,7,8,9,10]$. The hash library for converting string into signature value is \texttt{hashlib}. The number of repetitions of LSH is set to $T=10$. We note that the number of repetitions determines the memory and also the running time of the FLAN algorithm. A higher number of repetitions give us a higher quality normalization while a lower number gives us a faster algorithm. We set the threshold ratio $\alpha=0.2$ for removing low weight edges. Furthermore, we set the universe size to $U=U'=2^{32}$ and partition the space into 4 bins. The 2-universal hashing function we use in our experiments is $h(x)=(ax+b)\mod P$, where $a\sim[1,U],b\sim[0,U-1]$ and the prime number $P=2^{31}-1$. As there are several random functions used in FLAN, we fix a random seed value for reproducibility.
% comments from WSDM 2021 reviewer 2
% Section 3 seems to suggest that SHA256 is a 2-universal hash function, which I don’t believe is the case. Also cryptographic hash functions are quite slow compared to the hash function commonly used in the context of LSH or Sketches; for some pointers on the state of the art in string hashing see e.g.: https://courses.cs.washington.edu/courses/cse521/15sp/refs/thorup1.pdf

% P need to be prime. I don’t think the “2-universal” hash function described in Section 4.1. is, in fact, 2-universal: AFAIK, both a and b have to be odd numbers and P needs to be prime for this to hold.
\subsection{Comparison Details}
\begin{table*}
\small
\begin{tabular}{l|l|l}
\toprule
 &Pivot & Original words(Frequency)  \\\midrule
 small&toddler&toddler(408589), toddlers(53870), toddlera(25), toddlere(12), toddlerd(4), toddlert(3), \\
 &&  toddlersa(1),toddlero(1) \\
& months&months(435919), months+(332), 7months(33), 7months+(5), mmonths(5), monthsb(2), \\
&&1months(2), monthson(1)\\
&girls &girls(425439), sgirls(3), sgirl(2)\\
&newborn& newborn(258464), newborns(7719), newborn(6), +newborn(4), newbornâ(4), newbornn(4),\\
&&newborn+(3)\\
&clothes& clothes(213860), clothess(27), -clothes(2), clothesrl(1), (clothes5, 1), clothesc(1), clothesl(1),\\
&&clothesr(1) \\
\midrule
medium& with &with(347197), nwith(2), witht(2)\\
       &collar &collar(303697),collara(43), ccollar(5),collaras(3),collar5(2), gcollar(1),mcollar(1),wcollar(1),\\
       &&collar-(1) \\
& large & large(297583), larges(59), 1large(3), blarge(1), \\
& food & food(289124), foodn(8), foodno(1) \\
& medium & medium(196184), "medium(1), mmedium(1) \\
   \midrule 
large&sleeve & sleeve(4763366),sleevee(194),sleevev(60),sleeveer(6),sleeve–(5),+sleeve(5),sleeveh(2),\\
&&sleevevess(2), sleeveve(2)\\
& long &long(4541576), glong(7) \\
& t-shirt&t-shirt(4200960), t-shirt(4200204), t-shir(749), "t-shirt(3), .t-shirt(2), t-shirt0(1), t-shirt02(1) \\
&shirt & shirt(3741891), a-shirt(1593), -shirt(465), shirtl(69), shirth(23), y-shirt(13), eshirt(6), shirthy(1) \\
&womens&womens(3663167), ?womens(15), womensz(1) \\
twitter&sounds&sounds(5982), soundss(4)  \\
&yesterday&yesterday(5312), yesterdayl(1) \\
&shopping&shopping(3417), shoppingh(1) \\
&homework&  shopping(3417), shoppingh(1)\\
&unfortunately&  unfortunately(2002), unfortunately.(65), unfortunately...(14), unfortunately..(11),  \\
&&unfortunately....(2), unfortunately...i(2), unfortunately..i (1), unfortunately..im(1)\\
\bottomrule 	
\end{tabular}
\caption{Case study of LSH lexical normalization of words. All the words in the right column are mapped to the pivot words in the left column. The examples are picked from the vocabulary built from FLAN, the first one has the largest frequency with non-empty lexically similar components. FLAN has the ability to adjust to different distribution of the data.}\label{tab: appendix-case-study}	
\end{table*}

\noindent\textbf{Quality Comparison.} We evaluate the correction results from different algorithms by native speakers on Amazon Turk.
To measure the quality of the corrections by FLAN, we conduct a human evaluation study to evaluate the algorithms' performance. We first select 300 testing instance dataset that were corrected by either FLAN or the spell-correction method. Then we deploy the questionnaire to the AmazonTurk for native speaker to labels it. The evaluators did not know if a correction came from FLAN or the spell corrector, and each reviewer was tasked with labeling word corrections as either ``good", ``neutral'', ``bad'', and ``not sure''. We define a ``good" corrections as one that query is better for human understanding or one that eliminates unnecessary punctuation; ``neutral'' denotes a correction does not help to make the meaning of the query more clear, but does not hurt either, such as converting a word from plural to singular; ``bad'' corrections are those that make the query less coherent. Finally, we use ``not sure" to capture the remaining cases.  To give a quantitative result, we consider ``good", ``neutral'' as correct correction and regard ``bad'' and ``not sure'' as incorrect correction. The results are presented in Figure~\ref{tab:human}.

\noindent\textbf{Case Study.} In Table~\ref{tab: appendix-case-study}, All the words in the right column are mapped to the pivot words in the left column. The examples are picked from the vocabulary built from FLAN, the first one has the largest frequency with non-empty lexically similar components. FLAN has the ability to adjust to different distribution of the data.

We collect the statistics of the vocabulary produced by the FLAN method.
Figure~\ref{fig:cc} presents the number of connected components versus the size of connected components. The sizes of these connected components in all the datasets follow a power law. The points on the top left show that the majority of words have a limited number of lexical variants. The points on the bottom right show that there are some words with many variants.
\begin{figure}[!t]
\centering
\includegraphics[width=0.75\linewidth]{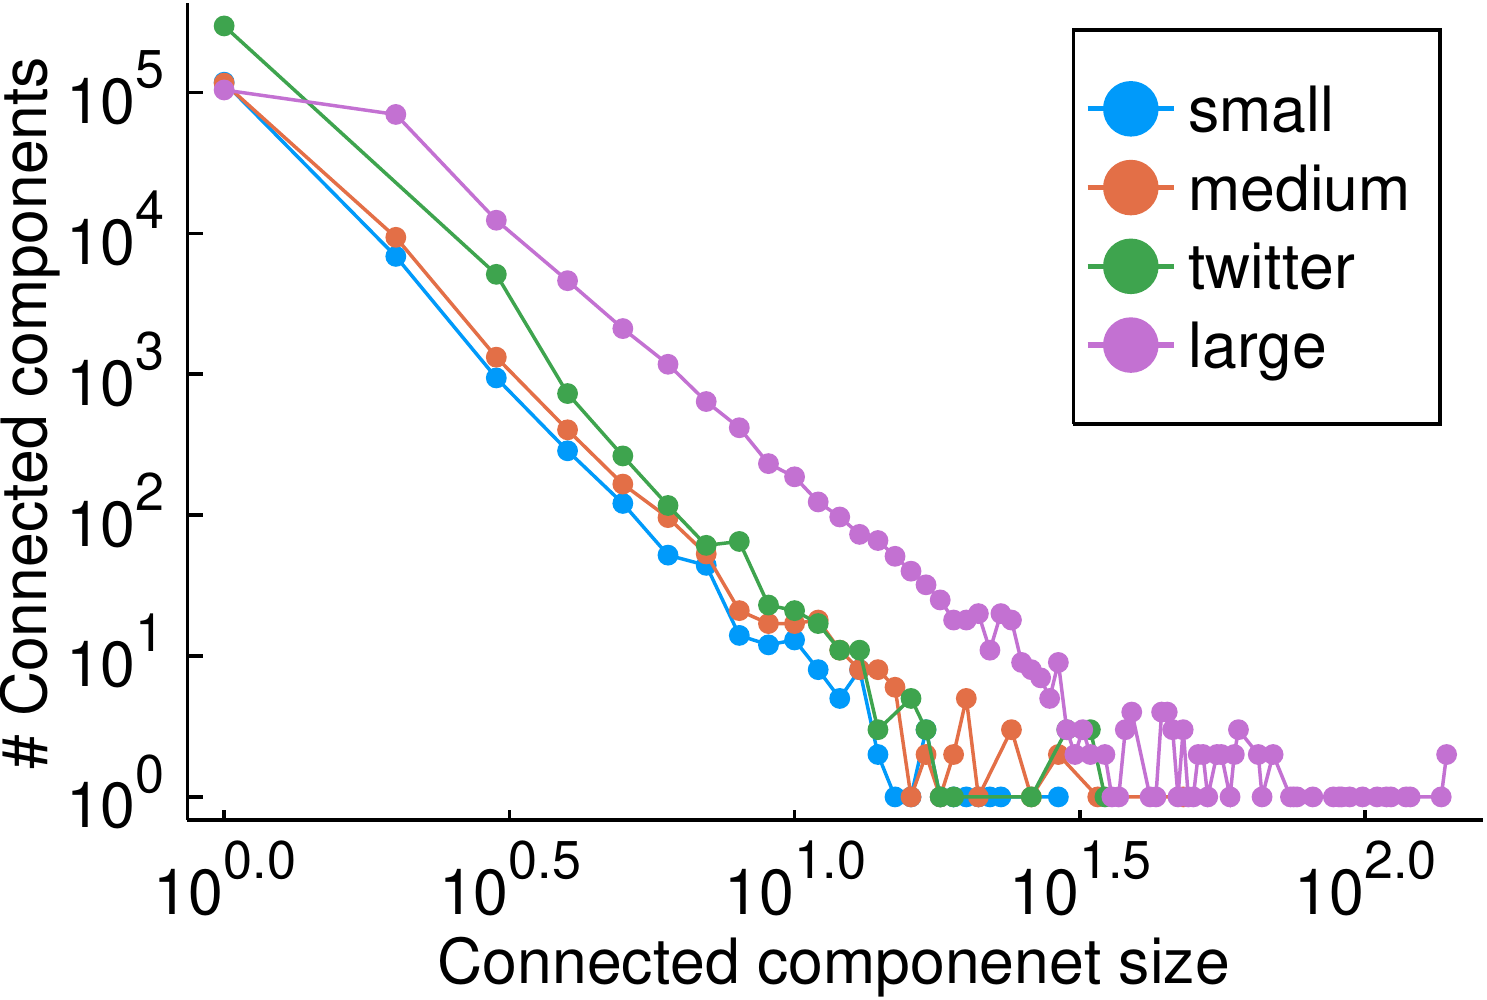}
\caption{The power-law distribution of connected components on all datasets. The top left points mean the majority of words have limited spelling errors. The bottom right points means users tend to make a various mistake for a tiny fraction of the words.}\label{fig:cc}
\end{figure}
